# Supplementary material for: Dense Dynamic Scene Reconstruction and Camera Pose Estimation from Multi-View Videos
Source: arXiv:2603.12064 source file (2026-10-05)
Supplement: Supplementary file 1 [file tab_multicam_video_tracking.tex]

\begin{table}[t]
    \centering
    \caption{Quantitative comparisons of camera pose on the \textit{MultiCamVideo}~\cite{bai2025recammaster} dataset.
    ``droid" and ``megasam" mean different matching modules we use during the tracking.
    $\dagger$:To avoid memory overflow, we sample images with interval=8 for VGGT~\cite{wang2025vggt}.
    Best results are \textbf{bolded}.}
    \begin{tabular}{lcccc}
         \toprule
         \textbf{Method} & \textbf{Interval} & ATE$\downarrow$ & RTE$\downarrow$ & RRE$\downarrow$ \\
         \midrule
         VGGT$^{\dagger}$~\cite{wang2025vggt} & 8 & 0.027 & 0.016 & 0.177 \\
         Fast3R~\cite{yang2025fast3r} &  & 0.144 & 0.056  & 1.948 \\
         CUT3R~\cite{wang2025continuous} & & 0.175 & 0.011 & 0.164 \\
         $\pi^{3}$~\cite{wang2025pi} & & 0.023 & 0.006 & 0.042 \\
         \hdashline
         % Ours (droid) & & 0.059 & 0.002 & 0.035 \\
         Ours & & \textbf{0.005} & \textbf{0.001} & \textbf{0.011} \\
         \bottomrule
    \end{tabular}
    \label{tab_supp:mvv_tracking}
\end{table}
