# Supplementary material for: Dense Dynamic Scene Reconstruction and Camera Pose Estimation from Multi-View Videos
Source: arXiv:2603.12064 source file (2026-10-05)
Supplement: Supplementary file 2 [file tab_robolab_tracking.tex]

\begin{table}[t]
\centering
\small
\setlength{\tabcolsep}{4pt}

\caption{Trajectory evaluation on the MultiCamRobolab datasets. $\dagger$: To avoid memory overflow, we sample images with interval=2 for Fast3R~\cite{yang2025fast3r} and $\pi^{3}$~\cite{wang2025pi} and interval=8 for VGGT~\cite{wang2025vggt}.
Best results are \textbf{bolded}.}
\resizebox{\linewidth}{!}{%
\begin{tabular}{lcccccccccc}
\toprule
\multirow{2}{*}{\textbf{Method}} & \multirow{2}{*}{\textbf{Interval}} &
\multicolumn{3}{c}{$\textbf{RoboDog}_{overlap}$} &
\multicolumn{3}{c}{$\textbf{RoboDog}_{non-overlap}$} &
\multicolumn{3}{c}{\textbf{RoboArm}} \\
\cmidrule(lr){3-5} \cmidrule(lr){6-8} \cmidrule(lr){9-11}
& & ATE$\downarrow$ & RTE $\downarrow$ & RRE$\downarrow$
& ATE$\downarrow$ & RTE $\downarrow$ & RRE$\downarrow$
& ATE$\downarrow$ & RTE $\downarrow$ & RRE$\downarrow$\\
\midrule
VGGT$^{\dagger}$~\cite{wang2025pi} & 8 & 0.024& 0.012 & 0.446 & 0.019 & 0.014 & 0.423 & 0.006 &  0.004 & 0.187\\
Fast3R$^{\dagger}$~\cite{yang2025fast3r} & 2 & 0.137 & 0.070 & 1.597  & 0.514 & 0.223 & 4.784 & 0.048 &  0.049 & 0.919 \\
${\pi^{3}}^{\dagger}$~\cite{wang2025pi} & 2 & 0.022 &  0.006 & 0.209 & \textbf{0.011} & 0.005 & 0.206 & \textbf{0.005} & 0.002 & 0.079  \\
CUT3R~\cite{wang2025continuous} & \ & 0.277 & 0.016 &  0.299 & 0.377 & 0.021 & 0.326 & 0.055  & 0.003  &  0.112 \\
% Ours (w/o) sp & 0.164 & 0.006 & 0.166 & 0.017 & \textbf{0.001} & 0.059 \\
% Ours (w/o) vggt init. & 0.497 & 0.016 & 0.224 & 0.026 & \textbf{0.001} & \textbf{0.058} \\
Ours & \ & \textbf{0.012} &  \textbf{0.003} & \textbf{0.157} & 0.034 & \textbf{0.003} & \textbf{0.148} & \textbf{0.005} & \textbf{0.001} & \textbf{0.059} \\
\bottomrule
\end{tabular}
}
\label{tab_supp:robolab_tracking}
\end{table}
